# Supplementary material for: AUBER: Automated BERT Regularization
Source: arXiv:2009.14409 source file (2020-09-30)
Supplement: Supplementary file 1 [file 080appendix2.tex]

\section{\method Definition and Proof}
\label{sec:FALCON_def_pro}
%We propose \method (FAst and Lightweight CONvolution), a novel convolution architecture that replaces standard convolution by applying EHP decomposition.
%
%\method is an efficient method with fewer parameters and computations than the standard convolution. 

\begin{definition}[\method]
\method is described as follows:
\begin{align}
\textbf{O}'_{h_i,w_j,n} &= \sum^{M}_{m=1} \textbf{P}_{m,n} \cdot \textbf{I}_{h_i,w_j,m} \label{eq:falcon_pw} \\
\textbf{O}_{h',w',n} &= \sum^{D}_{i=1} \sum^{D}_{j=1} \textbf{D}_{i,j,n} \cdot \textbf{O}'_{h_i,w_j,n} \label{eq:falcon_dw}
\end{align}
where $\textbf{I}$/$\textbf{O}'$/$\textbf{O}$ are the input/intermediate/output of convolution layer, respectively. $\textbf{P}$ is pointwise convolution kernel and $\textbf{D}$ is depthwise convolution kernel.
\end{definition}

\begin{lemma}
\method is derived by decomposing standard convolution kernel using EHP along output-axis (EHP-out).
\end{lemma}

\begin{proof}
%We describe the detailed derivation process as follows:
According to the definition of EHP along some axes, the kernel tensor of standard convolution $\textbf{K}$ can be decomposed into two tensors $\textbf{P} \in \mathbb{R}^{M \times N}$ and $\textbf{D}\in \mathbb{R}^{D \times D \times N}$ by EHP along output-axis:
\begin{align*}
\textbf{K}_{i,j,m,n} \approx \textbf{D}_{i,j,n} \cdot \textbf{P}_{m,n}
\end{align*}

Since EHP is the element-wise operation, it has commutative property.
Thus,
\begin{align}
\textbf{K}_{i,j,m,n} \approx \textbf{P}_{m,n} \cdot \textbf{D}_{i,j,n}
\label{eq:FALCON_kernel}
\end{align}
The decomposition procedure is demonstrated in Figure~\ref{fig:falcon}.

To approximate standard convolution kernel with fewer parameters, we substitute Equation~\ref{eq:FALCON_kernel} for Equation~\ref{eq:standardconv}. 
The convolution operation becomes:

\begin{align}
\textbf{O}_{h',w',n} = \sum^{D}_{i=1} \sum^{D}_{j=1} \sum^{M}_{m=1} \textbf{D}_{i,j,n} \cdot \textbf{P}_{m,n} \cdot \textbf{I}_{h_i,w_j,m}
\label{eq:falcon_long}
\end{align}

Equation~\ref{eq:falcon_long} is split into Equation~\ref{eq:falcon_pw_} and Equation~\ref{eq:falcon_dw_} by grouping summation.

\begin{align}
\textbf{O}'_{h_i,w_j,n} &= \sum^{M}_{m=1} \textbf{P}_{m,n} \cdot \textbf{I}_{h_i,w_j,m} \label{eq:falcon_pw_}
\end{align}
\begin{align}
\textbf{O}_{h',w',n} &= \sum^{D}_{i=1} \sum^{D}_{j=1} \textbf{D}_{i,j,n} \cdot \textbf{O}'_{h_i,w_j,n} \label{eq:falcon_dw_}
\end{align}

Equation~\ref{eq:falcon_pw_} and Equation~\ref{eq:falcon_dw_} are exactly the same as Equation~\ref{eq:falcon_pw} and Equation~\ref{eq:falcon_dw} under \method definition.
We conclude that \method is derived by decomposing standard convolution kernel using EHP along output-axis.
\end{proof}

\section{EHP-in Definition and Proof}
\label{sec:DSC_def_pro}

\begin{definition}[EHP-in]
EHP-in is described as follows:
\begin{align}
\textbf{O}'_{h',w',m} &= \sum^{D}_{i=1} \sum^{D}_{j=1} \textbf{D}_{i,j,m} \cdot \textbf{I}_{h_i,w_j,m} \label{eq:mobileconv_dw}\\
\textbf{O}_{h',w',n} &= \sum^{M}_{m=1} \textbf{P}_{m,n} \cdot \textbf{O}'_{h',w',m} \label{eq:mobileconv_pw}
\end{align}
where $\textbf{I}$/$\textbf{O}'$/$\textbf{O}$ are the input/intermediate/output of convolution layer, respectively. $\textbf{D}$ is depthwise convolution kernel and $\textbf{P}$ is pointwise convolution kernel.
\end{definition}

\begin{lemma}
EHP-in is derived by decomposing standard convolution kernel using EHP along input-axis (EHP-in).
\end{lemma}
%\begin{proof}
%Here we only briefly prove it.
%
%According to the definition of EHP along some axes, the kernel tensor of standard convolution $\textbf{K}$ can be decomposed into two tensors $\textbf{D} \in \mathbb{R}^{D \times D \times M}$ and $\textbf{P} \in \mathbb{R}^{M \times N}$ by EHP along output-axis:
%\begin{align}
%\textbf{K}_{i,j,m,n} = \textbf{D}_{i,j,n} \cdot \textbf{P}_{m,n}
%\label{eq:EHP-in_kernel}
%\end{align}
%
%Substitute the kernel tensor in Equation 1 with Equation~\ref{eq:EHP-in_kernel}, the convolutional operation becomes:
%\begin{align}
%\textbf{O}_{h',w',n} &= \sum^{M}_{m=1} \sum^{D}_{i=1} \sum^{D}_{j=1} \textbf{P}_{m,n} \cdot \textbf{D}_{i,j,m} \cdot \textbf{I}_{h_i,w_j,m} \label{mobileconv}
%\end{align}
%

%Proved.
%\end{proof}
\begin{proof}
According to the definition of EHP along some axes, the kernel tensor of standard convolution $\textbf{K}$ can be decomposed into two tensors $\textbf{D}\in \mathbb{R}^{D \times D \times M}$ and $\textbf{P} \in \mathbb{R}^{M \times N}$ by EHP along input-axis:
\begin{align}
\textbf{K}_{i,j,m,n} \approx \textbf{D}_{i,j,m} \cdot \textbf{P}_{m,n}
\label{eq:DSC_kernel}
\end{align}

The decomposition procedure is demonstrated in Figure~\ref{fig:mobileconv}.

To approximate standard convolution kernel with fewer parameters, we substitute Equation~\ref{eq:DSC_kernel} for Equation~\ref{eq:standardconv}. 
The convolution operation becomes:

\begin{align}
\textbf{O}_{h',w',n} &= \sum^{M}_{m=1} \sum^{D}_{i=1} \sum^{D}_{j=1} \textbf{P}_{m,n} \cdot \textbf{D}_{i,j,m} \cdot \textbf{I}_{h_i,w_j,m} 
\label{eq:mobileconv_long}
\end{align}

Equation~\ref{eq:mobileconv_long} is split into Equation~\ref{eq:falcon_pw_} and Equation~\ref{eq:falcon_dw_} by grouping summation.

\begin{align}
\textbf{O}'_{h',w',m} &= \sum^{D}_{i=1} \sum^{D}_{j=1} \textbf{D}_{i,j,m} \cdot \textbf{I}_{h_i,w_j,m} \label{eq:mobileconv_dw_}
\end{align}
\begin{align}
\textbf{O}_{h',w',n} &= \sum^{M}_{m=1} \textbf{P}_{m,n} \cdot \textbf{O}'_{h',w',m} \label{eq:mobileconv_pw_}
\end{align}

Equation~\ref{eq:mobileconv_dw_} and Equation~\ref{eq:mobileconv_pw_} are exactly the same as Equation~\ref{eq:mobileconv_dw} and Equation~\ref{eq:mobileconv_pw} under EHP-in definition.
We conclude that EHP-in is derived by decomposing standard convolution kernel using EHP along input-axis.

\end{proof}

\section{Compression Statistic on VGG16\_BN}
\begin{table*}[]
\centering
\caption{Compression statistics for all convolution layers in VGG16\_BN model. The number of parameters and FLOPs only consider the convolution operation. Bias, batch normalization, and ReLU activation function do not take into account. }
\label{tab:statistic_vgg16bn}
\begin{tabular}{lrlrl}
\toprule
Layer 		&\# of param	&			  	& \# of FLOPs 	 	&		  \\
\midrule
StConv1-1	& 1,728     	&             	& 89,915,392    		&         \\
FALCON1-1   	& 768       	& (2.25$\times$)	& 38,535,168    		& (2.33$\times$) \\
\midrule
StConv1-2	& 36,864    	&             	& 1,852,899,328 		&         \\
FALCON1-2   	& 4,672     	& (7.89$\times$)	& 234,422,272   		& (7.90$\times$) \\
\midrule
StConv2-1	& 73,728    	&             	& 926,449,664   		&         \\
FALCON2-1   	& 9,344     	& (7.89$\times$)	& 117,211,136   		& (7.90$\times$) \\
\midrule
StConv2-2	& 147,456   	&             	& 1,851,293,696 		&         \\
FALCON2-2   	& 17,536    	& (8.41$\times$)	& 219,971,584   		& (8.42$\times$) \\
\midrule
StConv3-1 	& 294,912   	&            	& 925,646,848   		&         \\
FALCON3-1	& 35,072    	& (8.41$\times$)	& 109,985,792   		& (8.42$\times$) \\
\midrule
StConv3-2 	& 589,824   	&            	& 1,850,490,880 		&         \\
FALCON3-2  	& 67,840    	& (8.69$\times$)	& 212,746,240   		& (8.70$\times$) \\
\midrule
StConv3-3	& 589,824   	&            	& 1,850,490,880 		&         \\
FALCON3-3  	& 67,840    	& (8.69$\times$)	& 212,746,240   		& (8.70$\times$) \\
\midrule
StConv4-1 	& 1,179,648 	&             	& 925,245,440   		&         \\
FALCON4-1   	& 135,680   	& (8.69$\times$)	& 106,373,120   		& (8.70$\times$) \\
\midrule
StConv4-2 	& 2,359,296 	&             	& 1,850,089,472 		&         \\
FALCON4-2 	& 266,752   	& (8.84$\times$)	& 209,133,568   		& (8.85$\times$) \\
\midrule
StConv4-3 	& 2,359,296 	&             	& 1,850,089,472 		&         \\
FALCON4-3  	& 266,752   	& (8.84$\times$)	& 209,133,568   		& (8.85$\times$) \\
\midrule
StConv5-1	& 2,359,296 	&             	& 462,522,368   		&         \\
FALCON5-1	& 266,752   	& (8.84$\times$)	& 52,283,392    		& (8.85$\times$) \\
\midrule
StConv5-2 	& 2,359,296 	&             	& 462,522,368   		&         \\
FALCON5-2	& 266,752   	& (8.84$\times$)	& 52,283,392    		& (8.85$\times$) \\
\midrule
StConv5-3	& 2,359,296 	&             	& 462,522,368   		&         \\
FALCON5-3	& 266,752   	& (8.84$\times$)	& 52,283,392    		& (8.85$\times$) \\
\midrule
\midrule
Total	& 14,710,464	&			  	& 15,360,178,176		&		  \\
		& 1,672,512 	& (8.80$\times$)	& 1,827,108,864 		& (8.41$\times$) \\
\bottomrule
\end{tabular}
\end{table*}

\section{ShuffleUnit Result}
\begin{table*}[]
\centering
\caption{\method performance compared with ShuffleUnit on CIFAR10 and CIFAR100. FW100 stands for the time of forward propagate 100 sample images.}
\label{tab:shuffle_cifar}
\begin{tabular}{lllrrrrr}
\toprule
Dataset  & Model  & ConvType    & Accuracy & \# of param & \# of FLOPs & Inf-Time(s)  & FW100(ms)\\
\midrule
CIFAR10  & VGG19  & StConv      					& 93.28\%  & 20.30M      & 398.70M     & 1.47 	 & 10.348   \\
         &        & FALCON      					& 93.23\%  & 2.56M       & 47.23M      & 0.95   & 4.883   \\
         &        & ShuffleUnit 2$\times$(g=2) 	& 91.77\%  & 2.74M       & 46.66M     & 1.82	 & 12.480    \\
         &        & ShuffleUnit 3$\times$(g=6) 	& 91.70\%  & 2.50M       & 39.32M   & 2.33   & 18.465  \\
         &        & ShuffleUnit 4$\times$(g=8) 	& 91.64\%  & 3.33M       & 52.42M   & 3.10   & 29.329  \\
\cline{2-8}         
         & ResNet & StConv      					& 93.27\%  & 21.29M      & 292.52M     & 1.58   & 12.718  \\
         &        & FALCON     					& 92.86\%  & 2.63M       & 46.33M      & 0.99   & 6.105   \\
         &        & ShuffleUnit 2$\times$(g=2) 	& 90.28\%  & 3.08M       & 49.78M   & 2.31	 & 17.402    \\
         &        & ShuffleUnit 2$\times$(g=4) 	& 89.21\%  & 1.95M       & 32.81M   & 2.24   & 18.038  \\
         &        & ShuffleUnit 3$\times$(g=12) 	& 88.71\%  & 2.60M       & 44.35M   & 3.36   & 29.398  \\
\midrule
CIFAR100 & VGG19  & StConv      					& 71.93\%  & 20.35M      & 398.75M     & 1.47   & 10.471  \\
         &        & FALCON      					& 71.55\%  & 2.61M       & 47.28M      & 0.96   & 4.928  \\
         &        & ShuffleUnit 2$\times$(g=2) 	& 69.31\%  & 2.79M       & 46.71M   & 1.59   & 12.490  \\
         &        & ShuffleUnit 3$\times$(g=6) 	& 68.87\%  & 2.55M       & 39.36M   & 2.25   & 18.452  \\
         &        & ShuffleUnit 4$\times$(g=8) 	& 69.82\%  & 3.38M       & 52.47M   & 3.33   & 29.323  \\
\cline{2-8}          
         & ResNet & StConv      					& 66.79\%  & 21.34M      & 292.57M     & 1.58   & 12.850  \\
         &        & FALCON      					& 68.99\%  & 2.67M       & 46.38M      & 0.98   & 6.085  \\
         &        & ShuffleUnit 2$\times$(g=2) 	& 65.25\%  & 3.17M       & 49.88M   & 2.26	 & 17.436    \\
         &        & ShuffleUnit 2$\times$(g=4) 	& 64.16\%  & 2.04M       & 32.90M   & 2.36   & 18.038  \\
         &        & ShuffleUnit 3$\times$(g=12) 	& 62.68\%  & 2.74M       & 44.49M   & 3.42   & 29.613  \\
\bottomrule
\end{tabular}
\end{table*}

\begin{table*}[]
\centering
\caption{\method performance compared to StConv, DSConv, and MobileConvV2. \method is initialized with EHP decomposition tensors of StConv kernel. All results are based on our implementation.}
\label{tab:perf_FALCON_old}
\begin{tabular}{lllrrr}
\toprule
Dataset                   & Model                   & ConvType         & Accuracy & \# of param & \# of FLOPs	\\
\midrule
\multirow{10}{*}{CIFAR10}  & \multirow{5}{*}{VGG19}  & StConv           & 93.28\%  & 20.30M      	 & 398.70M	\\
                          &                         & FALCON           & 93.23\%  & 2.56M  		 & 47.23M	\\
                          &         	& ShuffleUnit V2 1.25$\times$ 	  & 92.65\%  & 2.40M       & 48.52M		\\      
                          &         	& ShuffleUnit V2 1.375$\times$ 	  & 92.84\%  & 2.86M       & 58.24M		\\    
                          &                         & DSC              & 91.76\%  & 2.56M        & 48.02M	\\
                          &                         & MobileConvV2-0.5 & 92.58\%  & 2.67M        & 51.80M	\\
                          &        	& ShuffleUnit 2$\times$(g=2) 	  & 91.77\%  & 2.74M        & 46.66M	\\
\cline{2-6}
                          & \multirow{4}{*}{ResNet34} & StConv           & 93.27\%  & 21.29M       & 292.52M	\\
                          &                         & FALCON           & 92.86\%  & 2.63M   		 & 46.33M	\\
                          &         	& ShuffleUnit V2 1.25$\times$ 	  & 92.01\%  & 2.47M       & 42.74M		\\      
                          &         	& ShuffleUnit V2 1.375$\times$ 	  & 92.13\%  & 2.98M       & 51.30M		\\    
                          &                         & DSC              & 91.30\%  & 2.62M        & 38.41M	\\
                          &                        & MobileConvV2-0.5  & 90.61\%  & 2.55M        & 39.78M	\\
                          &        	& ShuffleUnit 2$\times$(g=2) 	  & 90.28\%  & 3.08M        & 49.78M	\\
\midrule
\multirow{10}{*}{CIFAR100} & \multirow{5}{*}{VGG19}  & StConv           & 71.93\%  & 20.35M      	& 398.75M	\\
                          &                         & FALCON           & 71.55\%  & 2.61M  		& 47.28M 	\\
                          &         	& ShuffleUnit V2 1.25$\times$ 	  & 72.41\%  & 2.45M       & 48.57M		\\      
                          &         	& ShuffleUnit V2 1.375$\times$ 	  & 72.42\%  & 2.91M       & 58.29M		\\    
                          &                         & DSC              & 68.47\%  & 2.61M      	& 48.07M		\\
                          &                         & MobileConvV2-0.5 & 68.31\%  & 2.71M       	& 51.85M		\\
                          &         	& ShuffleUnit 2$\times$(g=2) 	  & 69.31\%  & 2.79M       & 46.71M 	\\
\cline{2-6}                          
                          & \multirow{5}{*}{ResNet34} & StConv           & 66.79\%  & 21.34M      	& 292.57M	\\
                          &                         & FALCON           & 68.99\%  & 2.67M  		& 46.38M		\\
                          &         	& ShuffleUnit V2 1.25$\times$ 	  & 65.34\%  & 2.53M       & 42.80M		\\      
                          &         	& ShuffleUnit V2 1.375$\times$ 	  & 66.78\%  & 3.04M       & 51.36M		\\    
                          &                         & DSC              & 65.47\%  & 2.67M       	& 38.45M		\\
                          &                         & MobileConvV2-0.5 & 59.78\%  & 2.59M       	& 39.83M		\\
                          &         	& ShuffleUnit 2$\times$(g=2) 	  & 65.25\%  & 3.17M       & 49.88M		\\
\midrule
\multirow{10}{*}{SVHN}    & \multirow{5}{*}{VGG19}  & StConv           & 94.92\%  & 20.30M      	& 398.70M	\\
                          &                         & FALCON           & 94.22\%  & 2.56M  		& 47.23M		\\
                          &         	& ShuffleUnit V2 1.25$\times$ 	  & 94.01\%  & 2.40M       & 48.52M		\\      
                          &         	& ShuffleUnit V2 1.375$\times$ 	  & 94.54\%  & 2.86M       & 58.24M		\\    
                          &                         & DSC              & 94.00\%  & 2.56M      	& 48.02M		\\
                          &                         & MobileConvV2-0.5 & 93.11\%  & 2.67M       	& 51.80M		\\
                          &         	& ShuffleUnit 2$\times$(g=2) 	  & 93.54\%  & 2.74M       & 46.66M		\\
\cline{2-6}                          
                          & \multirow{5}{*}{ResNet34} & StConv         & 94.07\%  & 21.29M      	& 292.52M	\\
                          &                         & FALCON           & 94.03\%  & 2.63M  		& 46.33M		\\
                          &         	& ShuffleUnit V2 1.25$\times$ 	  & 94.23\%  & 2.47M       & 42.74M		\\      
                          &         	& ShuffleUnit V2 1.375$\times$ 	  & 94.32\%  & 2.98M       & 51.30M		\\                                               
                          &                         & DSC              & 88.62\%  & 2.62M       	& 38.41M		\\
                          &                         & MobileConvV2-0.5 & 90.38\%  & 2.55M       	& 39.78M		\\
                          &         	& ShuffleUnit 2$\times$(g=2) 	  & 92.99\%  & 3.08M       & 49.78M		\\
                          
\bottomrule
\end{tabular}
\end{table*}
